# Supplementary material for: Tensorized Automata: Algebraically Informed Representation Learning for Sequential Decision Making
Source: arXiv:2611.21514 source file (2026-11-16)
Supplement: Supplementary file 1 [file supplementary.tex]

\PassOptionsToPackage{capitalize}{cleveref}
\newcommand{\jmlrprehyperref}{\RequirePackage{xr-hyper}}
\documentclass[cleveref]{l4dc2027}
\usepackage{preamble}

\begin{document}

\title[Tensorized Automata: Supplementary Material]{\papertitle: Supplementary Material}
\maketitle



\appendix
\input{appendix/main}

\clearpage
\bibliography{main}

\end{document}
